# Supplementary material for: BOOTPLACE: Bootstrapped Object Placement with Detection Transformers
Source: arXiv:2503.21991 source file (2025-03-27)

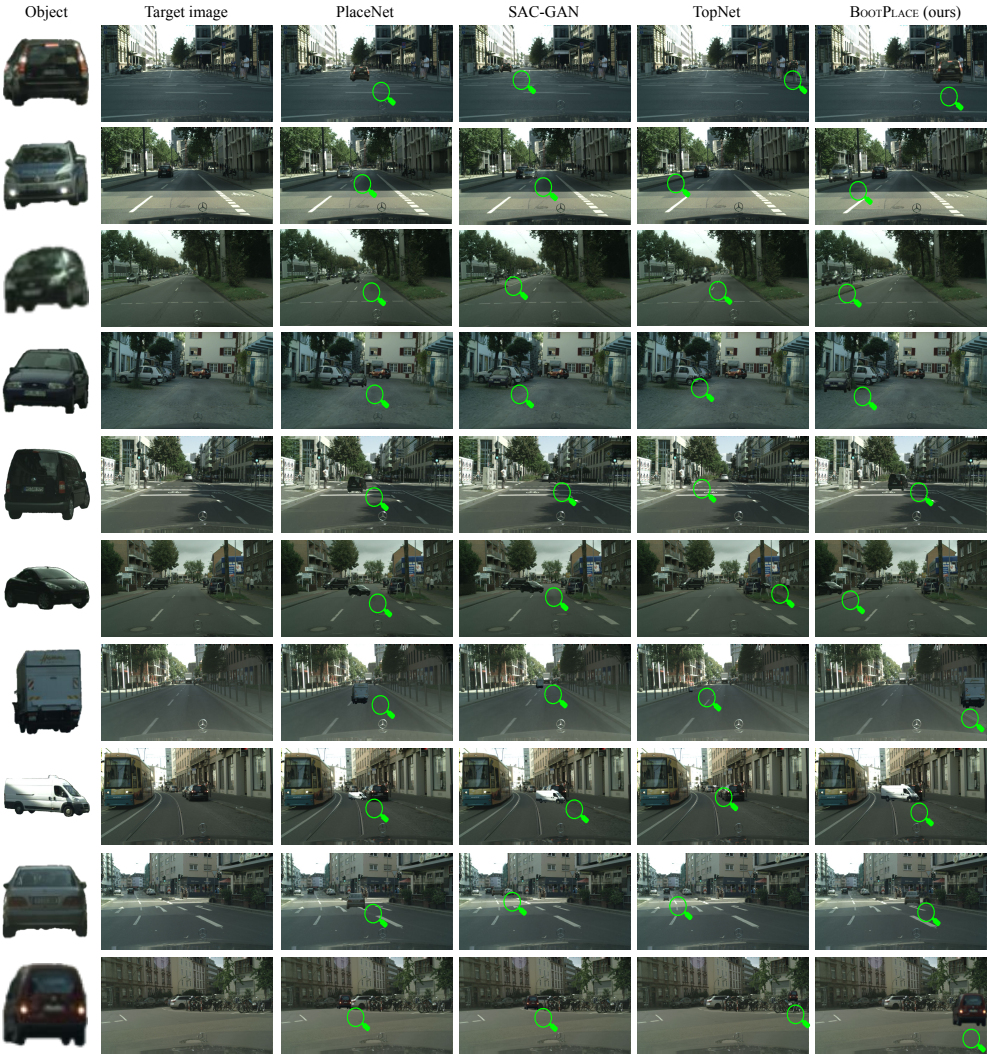

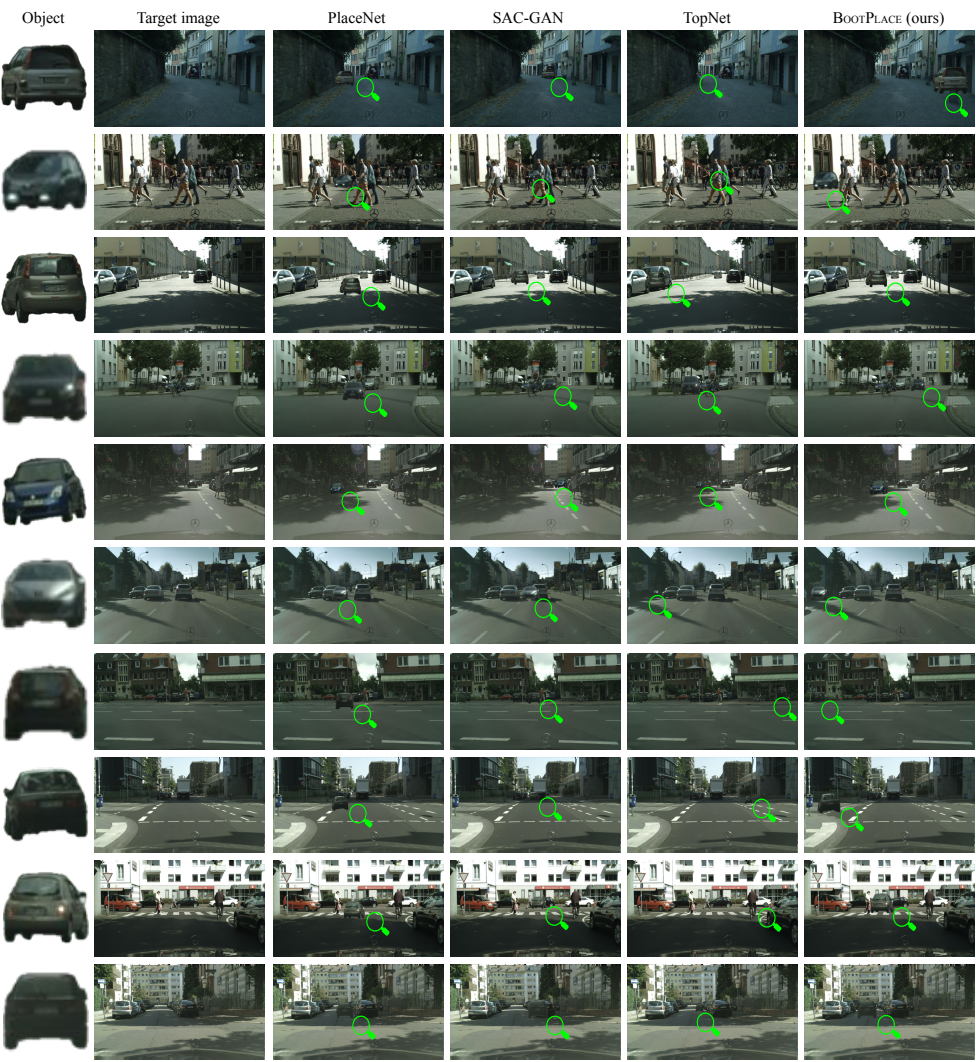

Supplement: Supplementary file 1 [file comp_vis_2_im.pdf]
